# Supplementary material for: Adaptive Importance Sampling for Efficient Stochastic Root Finding and Quantile Estimation
Source: arXiv:2102.10631 source file (2021-02-21)
Supplement: Supplementary file 1 [file ISvsSIS.tex]

%%%%%%%%%%%%%%%%%%%%%%%%%%%%%%%%%%%%%%%%%%%%%%%%%%%%%%%%%%%%%%%%%%%%%%%%%%%%
%% Author template for Operations Reseacrh (opre) for articles with no e-companion (EC)
%% Mirko Janc, Ph.D., INFORMS, mirko.janc@informs.org
%% ver. 0.95, December 2010
%%%%%%%%%%%%%%%%%%%%%%%%%%%%%%%%%%%%%%%%%%%%%%%%%%%%%%%%%%%%%%%%%%%%%%%%%%%%
%\documentclass[opre,blindrev]{informs3}
\documentclass[opre,nonblindrev]{informs3} % current default for manuscript submission

%\DoubleSpacedXI % Made default 4/4/2014 at request
\OneAndAHalfSpacedXI % current default line spacing
%%\OneAndAHalfSpacedXII
%%\DoubleSpacedXII

% If hyperref is used, dvi-to-ps driver of choice must be declared as
%   an additional option to the \documentclass. For example
%\documentclass[dvips,opre]{informs3}      % if dvips is used
%\documentclass[dvipsone,opre]{informs3}   % if dvipsone is used, etc.

%%% OPRE uses endnotes. If you do not use them, put a percent sign before
%%% the \theendnotes command. This template does show how to use them.
\usepackage{endnotes}
\let\footnote=\endnote

%

% Private macros here (check that there is no clash with the style)

% Natbib setup for author-year style
\usepackage{natbib}
 \bibpunct[, ]{(}{)}{,}{a}{}{,}%
 %
 %
 %
 %
 %

%% Setup of theorem styles. Outcomment only one.
%% Preferred default is the first option.
\TheoremsNumberedThrough     % Preferred (Theorem 1, Lemma 1, Theorem 2)
%\TheoremsNumberedByChapter  % (Theorem 1.1, Lema 1.1, Theorem 1.2)
\ECRepeatTheorems

\usepackage{pdflscape}
\usepackage{amsfonts}
\usepackage{setspace}
{\end{list}}
%%
%% Define \hangref environment for hanging indentation
%%

%%
%%
%%
%%
%% MATHEMATICS:
%%Special math symbols
%%
%% operators

\def\Var{{\rm Var}}

%%
%% bold face roman

\def\bX{{\bf X}}

\def\bealpha{\boldsymbol\alpha}
%% bold face Greek (incomplete)
\def\balpha{\mbox{\boldmath $\alpha$}}

%%
%% misc. Greek with hats

%%
%% caligraphy letters

%%
%% tt letters

%%
%% vec notation

%%
%% bold face numbers
\def\b1{{\bf 1}}

%%
%% \blot gives a square at end of formulas and proofs
%% (thanks to Marc Posner)
\def\blot{\quad {$\vcenter{\vbox{\hrule height.4pt
             \hbox{\vrule width.4pt height.9ex \kern.9ex \vrule
width.4pt}
             \hrule height.4pt}}$}}
%%
%% End of latexmacro

\usepackage{amssymb,latexsym}
\usepackage{amsmath}
\usepackage{graphics}
\usepackage{amsmath,amsfonts,amssymb,amsbsy,dsfont}
\usepackage{graphicx}
\usepackage{epstopdf}
\usepackage{multirow}
\usepackage{pstricks}
\usepackage{enumerate}
\usepackage{float}
\usepackage{bbm}
\usepackage{url}
\usepackage{color}
\usepackage{natbib}
\usepackage{booktabs}
\usepackage{algorithm}
\usepackage{algorithmicx}
\usepackage{algpseudocode}
%\usepackage{pseudocode}
%\geometry{left=2.0cm,right=2.0cm,top=2.5cm,bottom=2.5cm}
%\standard
%\usepackage[normalem]{ulem}
%\newcommand{\replace}[2]{\textcolor{blue}{\sout{#1}}
 %\textcolor{red}{{#2}}} % replace #1 with #2
%\newcommand{\delete}[1]{\textcolor{blue}{\sout{#1}}} % delete
%\newcommand{\ins}[1]{\textcolor{red}{\v{}{#1}}} % insert
%\newcommand{\cmt}[2]{\textcolor{blue}{({#1}: {#2})}} % comments

%\newtheorem{theorem}{Theorem}
%\newtheorem{lemma}{Lemma}
%\newtheorem{cor}{Corollary}[section]
%\newtheorem{proposition}{Proposition}
%\newtheorem{remark}{Remark}
%\newtheorem{assumption}{Assumption}
%\newtheorem{example}{Example}
%\newtheorem{condition}{Condition}
%\newtheorem{notation}{Notation}

%% Setup of the equation numbering system. Outcomment only one.
%% Preferred default is the first option.
\EquationsNumberedThrough    % Default: (1), (2), ...
%\EquationsNumberedBySection % (1.1), (1.2), ...

% In the reviewing and copyediting stage enter the manuscript number.
%\MANUSCRIPTNO{} % When the article is logged in and DOI assigned to it,
                 %   this manuscript number is no longer necessary

%%%%%%%%%%%%%%%%
\begin{document}
\graphicspath{{figures/}}
%%%%%%%%%%%%%%%%

\section{Importance Sampling vs. Sequential Importance Sampling}
In this section, we illustrate the advantage of sequential importance sampling (SIS) via a motivated case.
Suppose that $\theta\in\Re$ and $g(\theta)=\theta$. Furthermore, we assume that $f'(\theta^*)=1$.
Then, we know the asymptotic variance of both SA and SAA is $\Var(F(\bX,\theta^*))$.
Let
\begin{equation*}
\balpha^*(\theta) = \mathop{\arg\min}_{\bealpha} \Var_{\bX\sim P_{\bealpha}}\left( F(\bX,\theta)\ell(\bX,\balpha)\right).
\end{equation*}

If we want to apply optimal IS, the optimal IS parameter is given by $\balpha^*(\theta^*)$, and the corresponding asymptotic variance is given by
\begin{equation*}
\Var_{\bX\sim P_{\bealpha^*(\theta^*)}}\left( F(\bX,\theta^*)\ell(\bX,\balpha^*(\theta^*))\right)=\min_{\bealpha}\Var_{\bX\sim P_{\bealpha}}\left( F(\bX,\theta^*)\ell(\bX,\balpha)\right).
\end{equation*}
Notice that we do not know the value $\theta^*$, so we take a worst-case view, i.e., we will find $\balpha$ that solves 
\begin{equation*}
\min_{\bealpha}\max_{\theta^*}\Var_{\bX\sim P_{\bealpha}}\left( F(\bX,\theta^*)\ell(\bX,\balpha)\right),
\end{equation*}
which is the best worst-case asymptotic variance for the optimal IS.

On the other hand, we consider SIS. In both SAA and SA, we choose an optimal IS parameter at each time that we sample $\bX$, and obtain
\begin{equation*}
\balpha_{k+1}^*(\theta_{k}) = \mathop{\arg\min}_{\bealpha} \Var_{\bX\sim P_{\bealpha}}\left( F(\bX,\theta_k)\ell(\bX,\balpha)|\mathcal{F}_k\right).
\end{equation*}
As $k\rightarrow \infty$, under some mild conditions, we can prove that (see Lemma 6) 
\begin{equation*}
\balpha_{k+1}^*(\theta_{k})  \rightarrow \balpha^*(\theta^*),
\end{equation*}
and the asymptotic variance via SIS is given by
\begin{equation}\label{eq:asymvar_SIS_case1}
\Var_{\bX\sim P_{\bealpha^*(\theta^*)}}\left( F(\bX,\theta^*)\ell(\bX,\balpha^*(\theta^*))\right).
\end{equation}
Notice that \eqref{eq:asymvar_SIS_case1} is equivalent to
\begin{equation*}
\min_{\bealpha}\Var_{\bX\sim P_{\bealpha}}\left( F(\bX,\theta^*)\ell(\bX,\balpha)\right).
\end{equation*}
Since $\theta^*$ is generally unknown in advance, we take a worst-case view again. Particularly, the worst-case asymptotic variance for SIS among all possibilities of $\theta^*$ is
\begin{equation*}
\max_{\theta^*}\min_{\bealpha}\Var_{\bX\sim P_{\bealpha}}\left( F(\bX,\theta^*)\ell(\bX,\balpha)\right).
\end{equation*}
Then by using a standard weak duality, we have that 
\begin{equation*}
\max_{\theta^*}\min_{\bealpha}\Var_{\bX\sim P_{\bealpha}}\left( F(\bX,\theta^*)\ell(\bX,\balpha)\right) \leq \min_{\bealpha}\max_{\theta^*}\Var_{\bX\sim P_{\bealpha}}\left( F(\bX,\theta^*)\ell(\bX,\balpha)\right).
\end{equation*}
This result indicates that the worst-case asymptotic variance for applying SIS is at most that of applying optimal IS, and the SIS can generally outperform than optimal IS.

%%%%%%%%%%%%%%%%%
\end{document}
