# Supplementary material for: Adaptive Importance Sampling for Efficient Stochastic Root Finding and Quantile Estimation
Source: arXiv:2102.10631 source file (2021-02-21)
Supplement: Supplementary file 2 [file latexmacro.tex]

{\end{list}}
%%
%% Define \hangref environment for hanging indentation
%%

%%
%%
%%
%%
%% MATHEMATICS:
%%Special math symbols
%%
%% operators

%%
%% bold face roman

%%

%% bold face Greek (incomplete)

%%
%% misc. Greek with hats

%%
%% caligraphy letters

%%
%% tt letters

%%
%% vec notation

%%
%% bold face numbers
\def\b1{{\bf 1}}

%%
%% \blot gives a square at end of formulas and proofs
%% (thanks to Marc Posner)
\def\blot{\quad {$\vcenter{\vbox{\hrule height.4pt
             \hbox{\vrule width.4pt height.9ex \kern.9ex \vrule
width.4pt}
             \hrule height.4pt}}$}}
%%
%% End of latexmacro
